# Supplementary material for: Reflection Phase Shift of One-dimensional Plasmon Polaritons in Carbon Nanotubes
Source: arXiv:1910.02767 source file (2019-12-27)
Supplement: Supplementary file 1 [file supplemental_material.pdf]

# Supplementary Material: Reflection Phase Shift of One-dimensional Plasmon Polaritons in Carbon Nanotubes

Xingdong Luo,[1,2,†] Cheng Hu,[1,2,†] Bosai Lyu,[1,2,†] Liu Yang,[4,†]
Xianliang Zhou,[1,2] Aolin Deng,[1,2] Ji-Hun Kang[3,*] and Zhiwen Shi[1,2,*]
[1] *Key Laboratory of Artificial Structures and Quantum Control (Ministry of Education), Shenyang National Laboratory for Materials Science, School of Physics and Astronomy, Shanghai Jiao Tong University, Shanghai 200240, China*
[2] *Collaborative Innovation Center of Advanced Microstructures, Nanjing 210093, China*
[3] *Department of Optical Engineering, Kongju National University, Cheonan 31080, Korea*
[4] *School of Physics and Astronomy, University of Manchester, Manchester M13 9PL, United Kingdom*

## I. EXTRACTION OF RPS FROM EXPERIMENT

The carbon nanotube used in our experiment was synthesized according to the method in literatures[1]. This method was designed for synthesis of high-quality single-walled carbon nanotubes and ensure a high possibility that the nanotube end was closed. Considering it is the r-component of electric field that was detected in the experiment, from Eq.(3) in the main text we obtain the near-field intensity measured in FIG.2b is proportional to $|e^{ik_pz} + Re^{-ik_pz}|^2$. Taking account of $|R| \approx 1$, the maximum of the near-field intensity appears at $z = (\phi + 2\pi n)\frac{\lambda_p}{4\pi}$. This means that all required parameters to obtain the RPS are the wavelength of 1-D polaritons, and the distance between a peak and nanotube end. The position of the nanotube end is identified from the topography image (the left in FIG.2a in the main text) which is simultaneously obtained during the scanning. The wavelength of polaritons can be determined by measuring the distance between two neighboring peaks in FIG.2b. Eventually, the RPS can be calculated from the following equation,

$$\phi = \frac{4\pi \times z_{peak}}{2 \times (z_2 - z_3)} - 2\pi n \tag{S1}$$

$z_{peak}$ could be the coordinate of any one of the peaks. Note that $z < 0$ in our coordinate system. $z_2$ and $z_3$ are the coordinates of the second and third peaks, respectively. $n$ is an integer, which could be selected to set $\phi$ in the range $0 \sim 2\pi$.

## II. DETAILED DERIVATION OF THE ANALYTICAL MODEL

We will model the reflection problem in an extreme thin cylindrical shell, as shown in FIG.3b in the main text. The convention used for the harmonic time dependence in the analytical modeling is $e^{-i\omega t}$. Due to the motion of electrons is forbidden in the direction perpendicular to the carbon nanotube, the plasmon polaritons can almost exclusively generate electric current along the carbon nanotube, while the transverse electric current is nearly negligible. Considering the rotational symmetry of the carbon nanotube, the magnetic field of 1-D polaritons has the form

$$\mathbf{H}^L(\mathbf{r}) = h(r)e^{ik_pz}\mathbf{e}_\theta \tag{S2}$$

And the corresponding electric field reads

$$\begin{aligned}\mathbf{E}^L &= \frac{i}{\omega\varepsilon_0}\nabla \times \mathbf{H}^L \\ &= \frac{i}{\omega\varepsilon_0}[K_{pr}g(r)\mathbf{e}_z - ik_ph(r)\mathbf{e}_r]e^{ik_pz}\end{aligned} \tag{S3}$$

Using Maxwell's equations, one can obtain the following Helmholtz equation for $h(r)$,

$$\frac{\partial^2 h(r)}{\partial r^2} + \frac{1}{r}\frac{\partial h(r)}{\partial r} - \frac{1}{r^2}h(r) - (k_p^2 - k_0^2)h(r) = 0 \tag{S4}$$

For 1-D polaritons in carbon nanotube, $k_p \gg k_0$. The solution of $h(r)$ and $g(r)$ manifests as modified Bessel function.

$$h(r) = \begin{cases} CI_1(K_{pr}r) & r < r_0 \\ K_1(K_{pr}r) & r > r_0 \end{cases} \tag{S5}$$

$$K_{pr} = \sqrt{k_p^2 - k_0^2} \tag{S6}$$

And

$$g(r) = \begin{cases} CI_0(K_{pr}r) & r < r_0 \\ -K_0(K_{pr}r) & r > r_0 \end{cases} \tag{S7}$$

From the continuity of z-component of the electric field at $r = r_0$, we obtain

$$g(r_0 + 0) = g(r_0 - 0) \rightarrow C = -\frac{K_0(K_{pr}r_0)}{I_0(K_{pr}r_0)} \tag{S8}$$

*Electronic address: jihunkang@kongju.ac.kr; zwshi@sjtu.edu.cn

Considering it is the r-component of electric field that was detected and simulated in our experiment and simulation, we would seek for the launched-reflected polaritons interference in the following form

$$E_r^p(r,z) = \frac{k_p}{\omega\varepsilon_0} h(r)(e^{ik_p z} + Re^{-ik_p z}), \tag{S9}$$

$$H_\theta^p(r,z) = h(r)(e^{ik_p z} - Re^{-ik_p z}). \tag{S10}$$

$E_r^p(r,z)$ is the $r-$component of the electric field of polaritons, and $H_\theta^p(r,z)$ is the $\theta-$component of the magnetic field of polaritons. R is reflection coefficient. RPS of 1-D polaritons is defined as $\arg(R)$. For simplicity, the polaritons modes are considered to be the electromagnetic fields in the region $z < 0$,

$$E_r^<(r,z) \approx E_r^p(r,z) \tag{S11}$$

$$H_\theta^<(r,z) \approx H_\theta^p(r,z). \tag{S12}$$

We note that the reflection of the 1D polaritons induces evanescent waves near the end of the carbon nanotube. In the carbon nanotube region, those waves can be expanded in terms of an electromagnetic continuum of unbounded modes, as those of the 2D polaritons are introduced in refs.[2] and refs.[3]. In the 2D case, the unbounded modes modify the phase shift from $0.3\pi$ to $0.25\pi$ refs.[2], and similar improvement is expected in our 1D case by employing the unbounded modes.

Now let us represent the field in the region $z > 0$ in the form of the Fourier-Bessel expansion

$$H_\theta^>(r,z) = \int_0^{+\infty} kdke^{ik_z z} J_1(kr) f(k), \tag{S13}$$

$$E_r^>(r,z) = \frac{1}{\omega\varepsilon_0} \int_0^{+\infty} k_z kdke^{ik_z z} J_1(kr) f(k), \tag{S14}$$

$$k_z = \sqrt{k_0^2 - k^2}.$$

The boundary conditions in the plane $z = 0$ read

$$H_\theta^<(r,0) = H_\theta^>(r,0) \tag{S15}$$

$$E_r^<(r,0) = E_r^>(r,0) \tag{S16}$$

Combining equations from Eq.(S9) to Eq.(S16), we have

$$h(r)(1-R) = \int_0^{+\infty} kdkJ_1(kr) f(k) \tag{S17}$$

$$k_p h(r)(1+R) = \int_0^{+\infty} k_z kdkJ_1(kr) f(k) \tag{S18}$$

We project Eq.(S18) by $J_1(kr)$. After integration, we obtain

$$f(k) = (1+R)\frac{k_p}{k_z} \int_0^{+\infty} rdrJ_1(kr)h(r) \tag{S19}$$

where $f(k)$ is the expansion coefficient. Then we calculate the integral in Eq.(S19),

$$\int_0^{+\infty} rdrJ_1(kr)h(r) = \frac{r_0 G(k)}{k_p} \tag{S20}$$

$$G(k) = k_p \frac{kJ_2(kr_0)h_1 + K_{pr}J_1(kr_0)h_2}{k^2 + K_{pr}^2} \tag{S21}$$

where $G(k)$ is a dimensionless function.

$$h_1 = CI_1(K_{pr}r_0) - K_1(K_{pr}r_0) \tag{S22}$$

$$h_2 = CI_2(K_{pr}r_0) + K_2(K_{pr}r_0) \tag{S23}$$

We project Eq.(S17) by $h(r)$

$$(1-R)\int_0^{+\infty} rdrh^2(r) = \int_0^{+\infty} kf(k)dk \int_0^{+\infty} rdrJ_1(kr)h(r) \tag{S24}$$

Combining equations from Eq.(S19) to Eq.(S24), we have

$$\frac{1-R}{1+R} = \frac{r_0^2}{\int_0^{+\infty} rdrh^2(r)} \int_0^{+\infty} kdk \frac{G^2(k)}{k_z k_p} \tag{S25}$$

When $k_p \gg k_0$, some approximations can be taken to rewrite the expression of reflection coefficienct. $\frac{k}{k_z} = \frac{k}{\sqrt{k_0^2-k^2}} = \frac{k/k_p}{\sqrt{(k_0/k_p)^2-(k/k_p)^2}} \approx \frac{t}{\sqrt{-t^2}} \approx -i$, thereby the integral in Eq.(S25) can be approximated as

$$\int_0^{+\infty} kdk \frac{G^2(k)}{k_z k_p} \approx (-i)\int_0^{+\infty} dtG^2(tk_p) \tag{S26}$$

$$G(tk_p) \approx \frac{tJ_2(tk_p r_0)h_1 + J_1(tk_p r_0)h_2}{t^2+1} \tag{S27}$$

where $G(tk_p)$ is a dimensionless function.

$$h_1 \approx CI_1(k_p r_0) - K_1(k_p r_0)$$

$$h_2 \approx CI_2(k_p r_0) + K_2(k_p r_0)$$

And the rest integral in Eq.(S25) can be approximated as

$$\frac{r_0^2}{\int_0^{+\infty} rdrh^2(r)} \approx \frac{1}{\int_0^{+\infty} xdxh^2(xr_0)} \tag{S28}$$

$$h(xr_0) = \begin{cases} CI_1(k_p r_0 x) & r < r_0 \\ K_1(k_p r_0 x) & r > r_0 \end{cases}$$

Combining Eq.(S26) and Eq.(S28), we obtain an expression for reflection coeffcient $R$, which is the function of $k_p r_0$, namely $\lambda_p/D$, the relative size between polaritons wavelength and nanotube diameter.

$$\frac{1-R}{1+R} = \frac{(-i)\int_0^{+\infty} dtG^2(tk_p)}{\int_0^{+\infty} xdxh^2(xr_0)} = F(\frac{\lambda_p}{D}) \quad \text{(S29)}$$

## III. ENERGY FLOW OF THE EVANESCENT FIELD

Energy flow of electromagnetic field parallel to the nanotube in the region $z > 0$ reads

$$\begin{aligned}&\Sigma^{>}(z,t)_z \\ &= 2\pi \int_0^{+\infty} rdrRe\{E_r^{>}(r,z)e^{-i\omega t}\}Re\{H_\theta^{>}(r,z)e^{-i\omega t}\} \\ &= \Sigma_1(z,t) + \Sigma_2(z,t) + \Sigma_3(z,t) \quad \text{(S30)}\end{aligned}$$

$$\begin{aligned}&\Sigma_1(z,t) \\ &= \frac{4\pi r_0^2 \cos^2(\phi/2)}{\omega\varepsilon_0} \int_0^{k_0} \frac{k}{k_z} dkG^2(k) \quad \text{(S31)}\end{aligned}$$

$$\begin{aligned}&\Sigma_2(z,t) \\ &= \frac{4\pi r_0^2 \cos^2(\phi/2)}{\omega\varepsilon_0} \int_0^{k_0} \frac{k}{k_z} dkG^2(k)\cos(2k_z z - 2\omega t + \phi) \\ &\quad \text{(S32)}\end{aligned}$$

$$\begin{aligned}&\Sigma_3(z,t) \\ &= \frac{4\pi r_0^2 \cos^2(\phi/2)}{\omega\varepsilon_0} \int_{k_0}^{+\infty} \frac{k}{q_z} dkG^2(k)e^{-2q_z z}\sin(\phi - 2\omega t) \\ &\quad \text{(S33)}\end{aligned}$$

$$q_z = \sqrt{k^2 - k_0^2}$$

We can see $\Sigma_1(z,t)$ does not depend on time or position, so it represents the constant energy leakage due to the radiation of electromagnetic field. $\Sigma_2(z,t)$ fluctuates with $z$ and $t$, the time average of which is zero. Thus it represents energy flow of the "wave" part of the electromagnetic field. While $\Sigma_3(z,t)$ attenuates exponentially with $z$, which represents energy flow of evanescent part of the electromagnetic field.

$|R| \approx 1$ leads to the following simplification

$$1 - R = 2\sin(\phi/2)e^{i(\phi-\pi)/2} \quad \text{(S34)}$$

$$1 + R = 2\cos(\phi/2)e^{i\phi/2} \quad \text{(S35)}$$

$$\begin{aligned}\tan(\phi/2) &= \frac{ir_0^2}{Bk_p}\int_0^{+\infty} \frac{k}{k_z} dkG^2(k) \\ &= \frac{ir_0^2}{Bk_p}\int_0^{k_0} \frac{k}{k_z} dkG^2(k) + \frac{r_0^2}{Bk_p}\int_{k_0}^{+\infty} \frac{k}{q_z} dkG^2(k) \\ &= \frac{ir_0^2}{Bk_p}\Lambda_1 + \frac{r_0^2}{Bk_p}\Lambda_2 \quad \text{(S36)}\end{aligned}$$

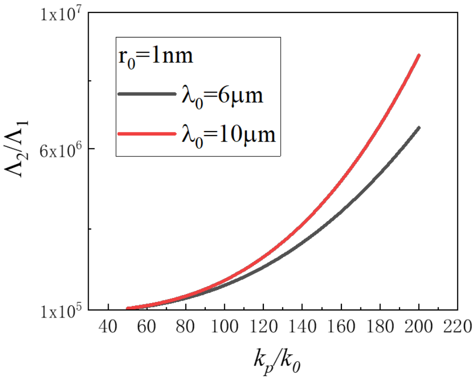


**Fig. S 1. Comparison between $\Lambda_2$ and $\Lambda_1$.**

$$B = \int_0^{+\infty} rdrh^2(r)$$

Fig. S1 show $\Lambda_1 \ll \Lambda_2$. Thus

$$\tan(\phi/2) \approx \frac{r_0^2}{Bk_p}\int_{k_0}^{+\infty} \frac{k}{q_z} dkG^2(k) \quad \text{(S37)}$$

Combining (S33) and (S37), we obtain

$$\begin{aligned}&\Sigma_3(z,t) \\ &= \frac{2\pi k_p B}{\omega\varepsilon_0} e^{-2q_z z}\sin\phi\sin(\phi - 2\omega t) \quad \text{(S38)}\end{aligned}$$

The time-average energy flow of launched polaritons at $z = 0$ plane can be calculated as

$$\begin{aligned}\bar{P}_0 &= \omega\int_0^{\frac{2\pi}{\omega}} dt \int_0^{+\infty} rdrE_r^L(r,0)\cos(\omega t)H_\theta^L(r,0)\cos(\omega t) \\ &= \frac{\pi k_p B}{\omega\varepsilon_0} \quad \text{(S39)}\end{aligned}$$

So the energy flow of evanescent field at $z = 0$ plane reads

$$P_{evane} = \Sigma_3(0,t) = \bar{P}_0[\cos(2\omega t) - \cos(2\omega t - 2\phi)] \quad \text{(S40)}$$

## IV. DISPERSION RELATION OF 1D PLASMON POLARITONS

Although there was no accurate optical conductivity of carbon nanotube calculated with consideration of luttinger liquid theory in previous literatures, a Drude-like model for the optical conductivity could be introduced to derive the dispersion relation of 1D plasmons with a decent accuracy. Firstly, the relation between $k_p$ and conductivity $\sigma_{zz}$ can be built by invoking the jump discontinuity in the magnetic field $H_\theta$ across the nanotube, $r = r_0$, which should be equal to the current $j_z = \sigma_{zz}E_z$.

$$\mathbf{e}_r \times (H_\theta(r_0+) - H_\theta(r_0-))\mathbf{e}_\theta = j_z\mathbf{e}_z = \sigma_{zz}E_z\mathbf{e}_z \quad \text{(S41)}$$

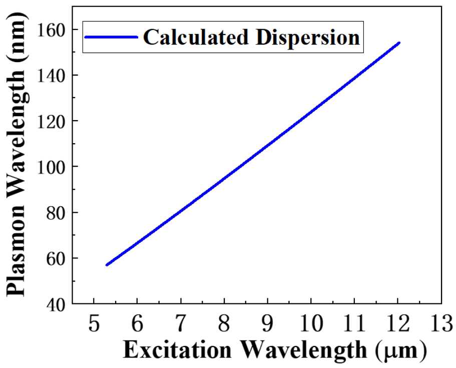


**Fig. S 2. Calculated dispersion of 1D plasmons in carbon nanotube.**

According to Equ.(S41), we get

$$\sigma_{zz} = \frac{K_1(K_{pr}r_0)I_0(K_{pr}r_0) + K_0(K_{pr}r_0)I_1(K_{pr}r_0)}{I_0(K_{pr}r_0)K_0(K_{pr}r_0)} \frac{i\omega\varepsilon_0}{K_{pr}} \tag{S42}$$

A Drude-like model for optical conductivity of carbon nanotube can be found in literatures[4, 5] ,

$$\sigma_{zz} = i\frac{2e^2 v_F \omega}{\pi^2 \hbar a(\omega^2 + \nu^2)} \tag{S43}$$

where $v_F \sim 0.8 \times 10^6 m/s$[6] and $\nu = (3 \times 10^{-12})^{-1}$[5] are the Fermi velocity and the relaxation frequency for a metallic carbon nanotube, respectively. Combining Equ.(S42)and Equ.(S43) can give the dispersion relation of 1D plasmon polaritons in metallic carbon nanotube,

$$\frac{2e^2 v_F}{\pi^2 \hbar a(\omega^2 + \nu^2)\varepsilon_0} = f(\lambda_p) \tag{S44}$$

where $f(\lambda_p) = \frac{K_1(K_{pr}r_0)I_0(K_{pr}r_0)+K_0(K_{pr}r_0)I_1(K_{pr}r_0)}{I_0(K_{pr}r_0)K_0(K_{pr}r_0)K_{pr}}$ is a function of plasmon wavelength $\lambda_p$. For $r_0 = 1$nm, excitation wavelength $\lambda_0 = 5.3\mu$m, $6.5\mu$m, $7.5\mu$m, $9.1\mu$m, and $12.0\mu$m, plasmon wavelength $\lambda_p$ =57nm, 74nm, 87nm, 111nm and 154nm, respectively. These results are quite agreed with the experimental results in FIG.3 of the main text.


[1] J. Kong, A. M. Cassell, and H. Dai, Chemical physics letters **292**, 567 (1998).
[2] J.-H. Kang, S. Wang, Z. Shi, W. Zhao, E. Yablonovitch, and F. Wang, Nano Letters **17**, 1768 (2017).
[3] A. Chaves, B. Amorim, Y. V. Bludov, P. A. D. Gonçalves, and N. Peres, Physical Review B **97**, 035434 (2018).
[4] G. Y. Slepyan, S. Maksimenko, A. Lakhtakia, O. Yevtushenko, and A. Gusakov, Physical Review B **60**, 17136 (1999).
[5] G. W. Hanson, IEEE Transactions on antennas and propagation **53**, 3426 (2005).
[6] S. Wang, F. Wu, S. Zhao, K. Watanabe, T. Taniguchi, C. Zhou, and F. Wang, Nano letters **19**, 2360 (2019).
